# Supplementary material for: Exchange functionals based on finite uniform electron gases
Source: arXiv:1612.06022 source file (2017-02-12)
Supplement: Supplementary file 1 [file A16.12.0186R_SuppMat.pdf]

# Supplementary Material for "Exchange functionals based on finite uniform electron gases"

Pierre-François Loos[1, 2, a)]

[1)] *Laboratoire de Chimie et Physique Quantiques, Université de Toulouse, CNRS, UPS, France*

[2)] *Research School of Chemistry, Australian National University, Canberra ACT 2601, Australia*

[a)] Electronic mail: pf.loos@anu.edu.au

TABLE I. Error (compared to UHF) in the exchange energy of the hydrogen-like ions for various LDA, GGA and GLDA functionals. The exact density is used for all calculations.

| Atom | LDA | GGAs | | | | GLDAs |
|---|---|---|---|---|---|---|
| | D30 | B88 | G96 | PW91 | PBE | GX |
| H | +0.0445 | +0.0027 | +0.0013 | +0.0056 | +0.0066 | −0.0179 |
| $He^{+}$ | +0.0889 | +0.0055 | +0.0026 | +0.0112 | +0.0131 | −0.0358 |
| $Li^{2+}$ | +0.1334 | +0.0082 | +0.0039 | +0.0168 | +0.0197 | −0.0537 |
| $Be^{3+}$ | +0.1779 | +0.0110 | +0.0052 | +0.0225 | +0.0262 | −0.0716 |
| $B^{4+}$ | +0.2223 | +0.0137 | +0.0064 | +0.0281 | +0.0328 | −0.0895 |
| $C^{5+}$ | +0.2668 | +0.0165 | +0.0077 | +0.0337 | +0.0394 | −0.1074 |
| $N^{6+}$ | +0.3112 | +0.0192 | +0.0090 | +0.0393 | +0.0459 | −0.1253 |
| $O^{7+}$ | +0.3557 | +0.0220 | +0.0103 | +0.0449 | +0.0525 | −0.1432 |
| $F^{8+}$ | +0.4002 | +0.0247 | +0.0116 | +0.0505 | +0.0590 | −0.1610 |
| $Ne^{9+}$ | +0.4446 | +0.0274 | +0.0129 | +0.0561 | +0.0656 | −0.1789 |

## REFERENCES

[1]K. P. Huber and G. Herzberg, *Molecular Spectra and Molecular Structure: IV. Constants of diatomic molecules* (van Nostrand Reinhold Company, 1979).

TABLE II. Error (compared to UHF) in the exchange energy of the helium-like ions for various LDA, GGA, GLDA, FMGGA and MGGA functionals.

| Atom | LDA | GGAs | | | | GLDA |
|---|---|---|---|---|---|---|
| | D30 | B88 | G96 | PW91 | PBE | GX |
| $H^-$ | +0.0790 | +0.0011 | +0.0009 | +0.0043 | +0.0065 | −0.0349 |
| He | +0.1727 | +0.0095 | +0.0047 | +0.0200 | +0.0239 | −0.0716 |
| $Li^+$ | +0.2594 | +0.0130 | +0.0050 | +0.0296 | +0.0353 | −0.1090 |
| $Be^{2+}$ | +0.3456 | +0.0224 | +0.0104 | +0.0451 | +0.0522 | −0.1392 |
| $B^{3+}$ | +0.4357 | +0.0284 | +0.0135 | +0.0571 | +0.0661 | −0.1753 |
| $C^{4+}$ | +0.5244 | +0.0337 | +0.0160 | +0.0682 | +0.0791 | −0.2112 |
| $N^{5+}$ | +0.6131 | +0.0391 | +0.0184 | +0.0793 | +0.0921 | −0.2470 |
| $O^{6+}$ | +0.7018 | +0.0445 | +0.0208 | +0.0904 | +0.1051 | −0.2828 |
| $F^{7+}$ | +0.7905 | +0.0499 | +0.0233 | +0.1015 | +0.1181 | −0.3186 |
| $Ne^{8+}$ | +0.8792 | +0.0553 | +0.0258 | +0.1126 | +0.1311 | −0.3543 |

| Atom | MGGAs | | | | | FMGGAs | |
|---|---|---|---|---|---|---|---|
| | M06-L | TPSS | revTPSS | MS0 | SCAN | MVS | PBE-GX |
| $H^-$ | +0.0002 | −0.0017 | −0.0007 | −0.0009 | −0.0001 | −0.0006 | +0.0010 |
| He | −0.0149 | +0.0004 | +0.0005 | +0.0001 | +0.0003 | +0.0002 | +0.0007 |
| $Li^+$ | −0.0207 | −0.0012 | −0.0010 | −0.0018 | −0.0015 | −0.0017 | −0.0010 |
| $Be^{2+}$ | −0.0272 | +0.0025 | +0.0021 | +0.0013 | +0.0010 | +0.0009 | +0.0006 |
| $B^{3+}$ | −0.0355 | +0.0026 | +0.0022 | +0.0016 | +0.0013 | +0.0013 | +0.0008 |
| $C^{4+}$ | −0.0427 | +0.0026 | +0.0022 | +0.0014 | +0.0012 | +0.0012 | +0.0007 |
| $N^{5+}$ | −0.0498 | +0.0025 | +0.0021 | +0.0014 | +0.0011 | +0.0011 | +0.0006 |
| $O^{6+}$ | −0.0569 | +0.0025 | +0.0021 | +0.0014 | +0.0010 | +0.0010 | +0.0005 |
| $F^{7+}$ | −0.0640 | +0.0024 | +0.0021 | +0.0013 | +0.0010 | +0.0001 | +0.0005 |
| $Ne^{8+}$ | −0.0711 | +0.0024 | +0.0021 | +0.0013 | +0.0009 | +0.0009 | +0.0004 |

TABLE III. Error (compared to UHF) in the exchange energy of the first-, second- and third-row atoms for various LDA, GGA, GLDA, FMGGA and MGGA functionals. The mean error (ME) and mean absolute error (MAE) per electron are also reported.

| Atom | LDA | GGAs | | | |
|---|---|---|---|---|---|
| | D30 | B88 | G96 | PW91 | PBE |
| H | +0.0591 | +0.0065 | +0.0042 | +0.0102 | +0.0116 |
| He | +0.1727 | +0.0095 | +0.0047 | +0.0200 | +0.0239 |
| Li | +0.2739 | +0.0115 | +0.0068 | +0.0257 | +0.0323 |
| Be | +0.3850 | +0.0174 | +0.0168 | +0.0311 | +0.0410 |
| B | +0.5182 | +0.0258 | +0.0252 | +0.0422 | +0.0569 |
| C | +0.6436 | +0.0325 | +0.0308 | +0.0514 | +0.0717 |
| N | +0.7669 | +0.0414 | +0.0362 | +0.0622 | +0.0895 |
| O | +0.9077 | +0.0335 | +0.0292 | +0.0558 | +0.0902 |
| F | +1.0398 | +0.0276 | +0.0213 | +0.0510 | +0.0939 |
| Ne | +1.1678 | +0.0253 | +0.0142 | +0.0498 | +0.1024 |
| Na | +1.3032 | +0.0398 | +0.0287 | +0.0661 | +0.1236 |
| Mg | +1.4542 | +0.0449 | +0.0375 | +0.0667 | +0.1337 |
| Al | +1.6137 | +0.0457 | +0.0329 | +0.0701 | +0.1474 |
| Si | +1.7737 | +0.0587 | +0.0415 | +0.0847 | +0.1717 |
| P | +1.9293 | +0.0705 | +0.0485 | +0.0979 | +0.1950 |
| S | +2.0974 | +0.0796 | +0.0530 | +0.1088 | +0.2168 |
| Cl | +2.2552 | +0.0834 | +0.0510 | +0.1140 | +0.2336 |
| Ar | +2.4082 | +0.0856 | +0.0460 | +0.1174 | +0.2488 |
| **ME** | 0.1120 | 0.0044 | 0.0033 | 0.0072 | 0.0118 |
| **MAE** | 0.0145 | 0.0008 | 0.0009 | 0.0013 | 0.0009 |

| Atom | MGGAs | | | | | FMGGAs | |
|---|---|---|---|---|---|---|---|
| | M06-L | TPSS | revTPSS | MS0 | SCAN | MVS | PBE-GX |
| H | −0.0069 | +0.0015 | +0.0013 | +0.0019 | +0.0017 | +0.0019 | +0.0014 |
| He | −0.0149 | +0.0004 | +0.0005 | +0.0001 | +0.0003 | +0.0002 | +0.0007 |
| Li | −0.0110 | −0.0047 | −0.0029 | −0.0047 | +0.0009 | +0.0021 | +0.0029 |
| Be | +0.0079 | −0.0065 | −0.0020 | −0.0047 | +0.0165 | +0.0206 | +0.0201 |
| B | +0.0079 | −0.0102 | −0.0022 | −0.0115 | +0.0176 | +0.0318 | +0.0250 |
| C | +0.0228 | −0.0041 | +0.0145 | −0.0178 | +0.0140 | +0.0378 | +0.0259 |
| N | +0.0304 | +0.0025 | +0.0315 | −0.0038 | +0.0143 | +0.0330 | +0.0135 |
| O | +0.0309 | −0.0161 | +0.0227 | −0.0249 | +0.0063 | +0.0441 | +0.0172 |
| F | +0.0419 | −0.0207 | +0.0355 | −0.0407 | −0.0099 | +0.0426 | +0.0086 |
| Ne | +0.0537 | −0.0228 | +0.0503 | −0.0294 | −0.0214 | +0.0252 | −0.0057 |
| Na | +0.0642 | −0.0128 | +0.0707 | −0.0289 | −0.0169 | +0.0405 | −0.0027 |
| Mg | +0.1075 | −0.0093 | +0.0916 | −0.0286 | −0.0137 | +0.0582 | +0.0234 |
| Al | +0.1121 | −0.0132 | +0.1065 | −0.0378 | −0.0264 | +0.0653 | +0.0054 |
| Si | +0.1353 | −0.0025 | +0.1353 | −0.0363 | −0.0275 | +0.0759 | −0.0051 |
| P | +0.1516 | +0.0073 | +0.1628 | −0.0241 | −0.0289 | +0.0775 | −0.0039 |
| S | +0.1654 | +0.0109 | +0.1822 | −0.0207 | −0.0299 | +0.0920 | −0.0128 |
| Cl | +0.1868 | +0.0151 | +0.2075 | −0.0198 | −0.0392 | +0.0979 | −0.0039 |
| Ar | +0.2005 | +0.0180 | +0.2319 | −0.0091 | −0.0443 | +0.0908 | −0.0358 |
| **ME** | 0.0066 | 0.0012 | 0.0056 | 0.0020 | 0.0019 | 0.0044 | 0.0016 |
| **MAE** | 0.0046 | 0.0018 | 0.0040 | 0.0038 | 0.0026 | 0.0014 | 0.0017 |

TABLE IV. Error (compared to the experimental value) in the atomization energy $E_{\mathrm{atoms}} - E_{\mathrm{molecule}}$ (in kcal/mol) of diatomic molecules at experimental geometry for various LDA, GGA, FMGGA and MGGA functionals. The mean error (ME) and mean absolute error (MAE) per electron are also reported. Experimental geometries are taken from Ref. 1.

| | LDA | GGA | | MGGAs | | | | | | | | | | |
|---|---|---|---|---|---|---|---|---|---|---|---|---|---|---|
| Exchange | D30 | B88 | PBE | M06-L | TPSS | revTPSS | SCAN | MVS | PBE-GX | | | | | |
| Correlation | VWN5 | LYP | PBE | M06-L | TPSS | revTPSS | SCAN | MVS | PBE | LYP | TPSS | revTPSS | regTPSS | SCAN |
| $H_2$ | −9.6 | −6.0 | −1.2 | −0.7 | −9.5 | −11.1 | −2.3 | −4.2 | −1.4 | −7.8 | −9.8 | −2.1 | −3.8 | −5.4 |
| LiH | −4.7 | −2.1 | +2.5 | −4.6 | −3.1 | −5.1 | +3.7 | +0.5 | +4.0 | −1.7 | −3.7 | +3.1 | +1.0 | −1.0 |
| BeH | −13.2 | −10. | −8.5 | −12.4 | −13.3 | −14.1 | −10.6 | −13.5 | −13.0 | −14.1 | −14.8 | −13.1 | −13.6 | −14.2 |
| $Li_2$ | +0.3 | +3.2 | +3.8 | −2.8 | +1.1 | +0.3 | +9.0 | +5.7 | +9.2 | +5.6 | +4.1 | +8.5 | +6.5 | +6.6 |
| HF | −26.7 | −5.6 | −6.6 | −0.3 | −3.6 | −1.7 | −9.2 | −1.8 | −5.7 | −9.5 | −10.3 | −6.0 | −6.6 | −6.3 |
| LiF | −17.9 | −2.1 | −0.6 | −2.0 | +2.5 | +3.4 | −1.1 | +4.2 | +1.5 | −0.6 | −1.5 | +1.1 | −0.9 | −2.6 |
| CN | −41.9 | −14.0 | −20.2 | +21.4 | −5.7 | −5.0 | −6.7 | −0.2 | −8.2 | −5.3 | −4.8 | −8.1 | −5.9 | −6.7 |
| $N_2$ | −41.3 | −14.4 | −17.7 | +1.2 | −2.0 | −3.0 | +2.7 | +6.6 | −1.6 | +2.3 | +2.6 | −1.8 | +2.3 | −4.2 |
| CO | −41.8 | −4.8 | −11.8 | −1.4 | +2.9 | +3.7 | −9.8 | +2.5 | −11.9 | −10.1 | −9.9 | −11.9 | −8.3 | −9.9 |
| NO | −47.8 | −15.6 | −21.3 | −0.7 | −5.4 | −5.4 | −4.2 | −0.4 | −7.4 | −5.0 | −4.7 | −7.5 | −6.2 | −7.1 |
| $O_2$ | −56.3 | −16.8 | −25.1 | −5.4 | −8.2 | −7.0 | −18.6 | −9.1 | −20.2 | −19.4 | −19.0 | −20.1 | −20.4 | −16.9 |
| $F_2$ | −41.0 | −12.0 | −16.1 | −0.2 | −9.1 | −10.5 | −6.0 | −0.5 | −8.1 | −7.6 | −7.7 | −8.2 | −8.1 | −8.0 |
| CH | −12.3 | −5.6 | −4.7 | −2.8 | −7.3 | −7.5 | −0.3 | −1.8 | −2.3 | −4.5 | −5.3 | −2.6 | −0.9 | −4.2 |
| NH | −16.2 | −10.3 | −9.3 | −3.4 | −11.0 | −10.9 | −0.9 | −5.8 | −2.7 | −4.8 | −5.5 | −3.1 | −3.0 | −4.8 |
| OH | −22.6 | −8.2 | −8.4 | −2.7 | −5.2 | −2.5 | −5.3 | −7.3 | −6.1 | −9.4 | −10.2 | −6.5 | −6.8 | −7.5 |
| HCl | −17.7 | −1.7 | −3.7 | −3.9 | −4.2 | −3.4 | −7.4 | −2.7 | −7.7 | −11.5 | −12.3 | −7.9 | −7.3 | −6.8 |
| $Na_2$ | −3.5 | −1.0 | −1.0 | −3.4 | −2.2 | −2.4 | +4.9 | +2.9 | +5.5 | +2.6 | +1.3 | +4.9 | +3.2 | +2.5 |
| $Si_2$ | −18.5 | −1.6 | −6.7 | −5.9 | −1.3 | −2.1 | −7.1 | −0.4 | −6.5 | −5.7 | −5.4 | −6.5 | −5.7 | −8.9 |
| $P_2$ | −25.3 | −3.7 | −3.7 | +2.9 | +1.4 | −1.0 | −0.6 | +6.4 | −1.7 | +0.4 | +0.5 | −2.0 | +0.5 | −4.1 |
| $S_2$ | −31.8 | −3.8 | −11.8 | −7.5 | −5.7 | −6.1 | −15.0 | −6.2 | −18.7 | −18.6 | −18.1 | −18.4 | −18.2 | −13.8 |
| $Cl_2$ | −24.2 | +1.3 | −6.6 | −3.3 | −2.4 | −3.7 | −6.7 | +0.7 | −10.6 | −10.3 | −10.1 | −10.4 | −10.2 | −6.1 |
| NaCl | −5.8 | +6.5 | +3.9 | −12.2 | +2.1 | +2.1 | −6.1 | +2.1 | −7.6 | −8.9 | −9.6 | −7.8 | −5.1 | −6.0 |
| SiO | −30.2 | −1.7 | −2.8 | +4.0 | +6.0 | +7.2 | −2.7 | +5.8 | −2.5 | −1.5 | −1.7 | −2.8 | −1.2 | −5.4 |
| SC | −30.7 | −1.1 | −8.4 | −2.1 | +1.2 | +1.2 | −8.1 | +3.7 | −10.2 | −8.9 | −8.6 | −10.1 | −7.0 | −6.8 |
| SO | −40.3 | −7.5 | −13.9 | −2.0 | −3.1 | −2.2 | −12.3 | −5.0 | −15.2 | −14.6 | −14.4 | −15.1 | −15.6 | −13.0 |
| ClO | −38.8 | −8.9 | −15.7 | −2.6 | −6.2 | −6.1 | −7.4 | −4.2 | −11.2 | −10.5 | −10.3 | −11.1 | −12.0 | −8.5 |
| **ME** | 1.8 | 0.6 | 0.7 | 0.4 | 0.6 | 0.6 | 0.5 | 0.4 | 0.6 | 0.6 | 0.7 | 0.8 | 0.6 | 0.6 |
| **MAE** | 3.7 | 1.2 | 1.2 | 1.2 | 1.1 | 1.2 | 0.9 | 0.7 | 1.2 | 1.1 | 1.3 | 1.5 | 1.1 | 1.0 |
